# Supplementary material for: Hierarchical Coded Matrix Multiplication
Source: arXiv:1907.08818 source file (2019-07-20)
Supplement: Supplementary file 1 [file Appendix.tex]

\section{Appendix}
\subsection{Proof of Thm.~\ref{thm.expected}}
\label{apn:1}
Let $T_1,\ldots, T_{\ND}$ be independent shifted exponential random variables with scale parameter $\mu$ and shift parameter $\alpha$, that denote the respective finishing time of the $n$ workers. Let $T_{n:\ND}$ be the $n$th order statistics and $\tau$ be the finishing time (i.e., at least $\DM_l$ subtasks finish every layer for all $l \in [\LY]$). Then the average finishing time is, 
\begin{align}\label{eqn:avg.finish}
	\mathbb E[\tau] \leq \max_{l\in[\LY]} \frac{l}{\DM} \mathbb E[T_{\DM_l:\ND}].
\end{align}  
We note that the expected value of the $\DM_l$th statistic of $T_1,\ldots, T_{\ND}$ is \cite{SPEEDUP:TIT17}[Eq. 11],
\begin{align}\label{eqn:expected.finish}
	\mathbb E[T_{\DM_l:\ND}] = \alpha + \sum_{i=\ND-\DM_l+1}^{\ND} \frac{\mu}{\i} \approx \alpha + \mu \log\left( \frac{\ND}{\ND-\DM_l}\right).
\end{align}
By using~(\ref{eqn:avg.finish}) and~(\ref{eqn:expected.finish}) we arrive  at Thm.~\ref{thm.expected}.

\subsection{Proof to optimizing $\{\DM_l \}_{l \in [\LY]}$}
\label{apn:2}
 The resulting optimization problem is to use~(\ref{eqn:expected.finish}) in the place of the objective in optimization problem, considering integer constraints on the $\DM_l$. Other constraints are obtained by the relationship among the parameters of our scheme. If we again relax the integer constraints the result is a piecewise min-max convex-concave optimization problem.  We can express the problem as the following. To solve we use barrier methods.
\begin {mini}
%\label{eqn:optimization.linear}
{z,\{\DM_l\}}{z}{\label{eqn:z.2}}{}
	\addConstraint{\DM=\sum_{l=1}^{\LY}\DM_l, \;\;\forall l \in [\LY]}	
\addConstraint{l\Big(\alpha + \mu \log \Big(\frac{\ND}{\ND-\DM_l}\Big)\Big) \leq z \DM,\;\; \forall l \in [\LY]}
\addConstraint{\DM_{l-1} \leq \DM_l ,\;\; \forall l \in [\LY]}
\addConstraint{\DM_l \leq \ND, \DM_l \in \mathbb Z^+\;\; \forall l \in [\LY]}
\end{mini}

We note that above method may be appropriate for small t where the large deviation bounds used
in~\cite{HIER:ISIT18} may be loose.
